# Supplementary material for: Electronic Thermal Conductivity Measurements in Intrinsic Graphene
Source: arXiv:1303.2390 source file (2013-06-27)
Supplement: Supplementary file 1 [file Yigen_Champagne_SM_PRB_4.pdf]

# Electronic Thermal Conductivity Measurements in Intrinsic Graphene

S. Yigen, V. Tayari, J. O. Island, J. M. Porter, and A. R. Champagne*
*Department of Physics, Concordia University, Montréal, Québec, H4B 1R6, Canada*
*E-mail: a.champagne@concordia.ca

## Supplemental Material

### Supplemental material contents

1. **Dimensions and $R$-$V_G$ data for Sample C**
   **Figure S1:** Sample C
2. **Upper bound for contact resistance**
   **Figure S2:** Upper bound for contact resistance of Sample A
3. **Mean-free path in the nearly intrinsic regime**
4. **Joule self-heating data for Samples B and C**
   **Figure S3:** Self-heating ($R$ vs $V_B$ and $T_e$ vs $V_B$ for Sample B)
   **Figure S4:** Self-heating ($R$ vs $V_B$ and $T_e$ vs $V_B$ for Sample C)
5. **Electron-electron scattering length**
   **Figure S5:** Mesoscopic conductance oscillation in Sample B.
6. **Error analysis**
7. **Specific heat calculation**
8. **Electron cooling length estimate**

### 1. Dimensions and $R$-$V_G$ data for Sample C

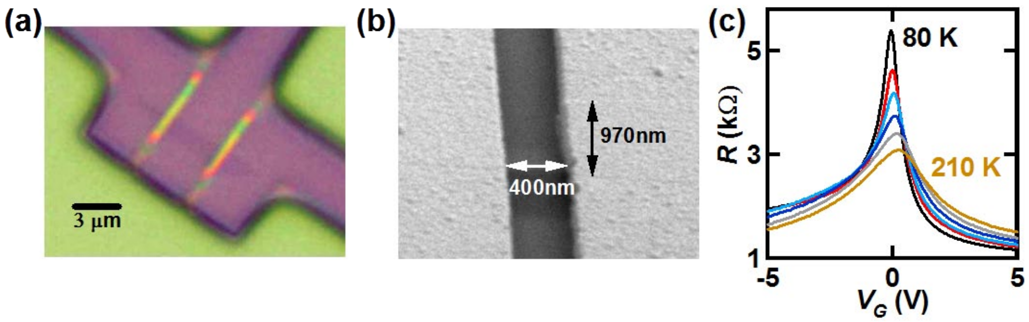


Figure S1: Sample C. (a) Optical image of three e-beam lithographically defined contacts (purple) on a graphene flake (dark purple). The two left electrodes connect Sample C, and the two right ones Sample A. (b) SEM of Sample C after the measurements were completed. The gold contacts are smooth and show the length of Device C (400 nm). The width of Device C can be inferred from the contrast of graphene under the gold (970 nm). The suspended section of Device C is not visible as it was damaged after the measurements were completed. (c) The $R$-$V_G$ data for Sample C at several $T$, after current annealing, showing a low charge impurity disorder $n^* = 2.2 \times 10^{10}$ cm$^{-2}$.

## 2. Upper bound for contact resistance

An upper bound for the contact resistance, $R_C$, of our devices can be extracted from the two-point $R$-$n_G$ curves. The data for Sample A is shown in Fig. S2. We fit the data with the expression [S1] $R = R_0 + \left(\frac{L}{W}\right)\frac{1}{n_G \mu}$ where $R_0$ is the resistance due to neutral scatterers plus $R_C$, $L$ is the length of the device, $W$ the width, $n_G$ the charge density induced by $V_G$, $\mu$ the mobility, and $e$ the electron's charge. We fit the data at $T = T_e$ = 100 K, and for ($V_G$ - $V_D$) > 1.3 V to avoid the thermal smearing around the Dirac point, $V_D$. The fit for the hole (electron) regime is shown as a light blue (red) dashed line in Fig. S2(a). The extracted mobility for Sample A in the doped regime is $\mu \approx 8.5 \times 10^4$ cm$^2$ V.s at 100 K, and $R_0 \approx 682 \pm 53$ and $1135 \pm 80$ Ω for hole and electron doping respectively. Panel (b) show the conductance, $G = 1/R$, for Sample A before the series resistance $R_0$ is subtracted (black line) and after $R_0$ is subtracted for the hole (light blue) and electron (red) doped data. The corrected conductance depends linearly on the gate induced charge density, $n_G$.

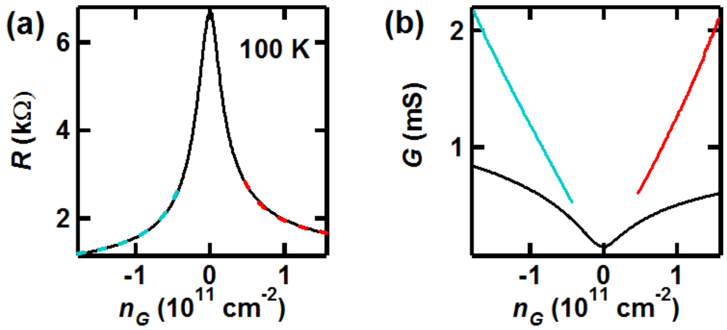


Figure S2: Upper bound for contact resistance of Sample A. (a) $R$-$n_G$ data at 100 K for Sample A. The light blue and red dashed lines are fits as described in the text from which the total series resistance, $R_0$, is extracted. (b) The same $G$-$n_G$ data as in panel (a), before (black line) and after (blue and red lines) subtracting $R_0$.

## 3. Mean-free path in the nearly intrinsic regime

To extract an approximate elastic mean free path, $l$, for charge carriers when the chemical potential is close to the Dirac point, we consider doping due to impurities, $n^*$, and thermally activated electron-hole pairs, $n_{th} = \left(\frac{\pi}{6}\right)\left(\frac{k_B T}{\hbar v_F}\right)^2$, where $k_B$ is Boltzmann's constant, $T$ the lattice temperature, $v_F$ = $10^6$ m/s the Fermi velocity. The total charge carrier density is [S2]

$$n_{tot} = n + p = \sqrt{n_G^2 + 4\left[\left(\frac{n^*}{2}\right)^2 + n_{th}^2\right]} \quad \text{(S1)}$$

where $n_G$ is the charge density induced by the gate electrode. For instance, at $T = 100$ K we find $n_{tot}(100\,K)$ = 2.4, 2.5 and 2.8 x $10^{10}$ cm$^{-2}$ for Samples A, B and C. We calculate the charge carrier mobility $\mu = \frac{\sigma}{n_{tot} e}$ , where $\sigma$ is the charge conductivity. At $T$

= 100 K, $\mu$ = 4.1 (4.8), 2.9 (3.6), and 2.0 (2.7) x $10^4$ $cm^2$/V.s using $R_c = 0$ ($R_{o-Dirac}$) for Samples A, B and C respectively. The mobility decreases with $T$ for all samples. From the mobility, we extract the mean-free path of the carriers as,

$$l = \sqrt{\frac{n_{tot}}{\pi}} \frac{h\mu}{2e} \tag{S2}$$

At $T$ = 100 K, we find $l$ = 74 (87), 54 (67), 39 (52) nm for A, B and C, which is several times shorter than the size of the samples.

## 4. Additional Joule self-heating data for Samples B and C

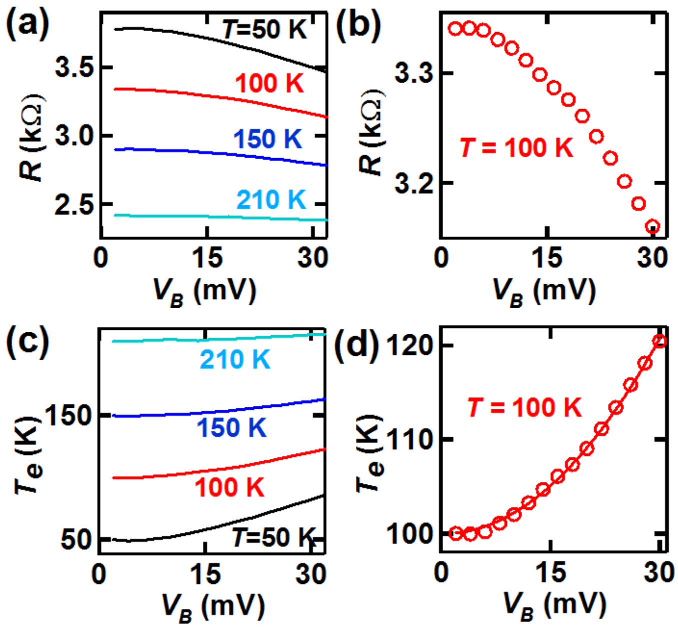


Figure S3: Electron heating for Sample B. (a) $R$ vs $V_B$ at $T$ = 50, 100, 150, 210 K at $V_G$ = 0.0 V ≈ $V_D$. (b) Zoom-in on the 100 K data. Joule heating due to $V_B$ raises the flake's average $T_e$ above $T$. $T_e$ is extracted using Fig. 2(a). Panels (c) and (d) show $T_e$ vs $V_B$ in Sample B at several $T$, and at $T$ = 100 K respectively. All of our $K_e$ data is extracted with $V_B \lesssim 30$ mV. The solid line in panel (d) is a power law fit $T_e = 100 + BV_B^x$, and we find $x$ = 2.02 ± 0.04, as expected for Joule heating over a small $T_e$ range.

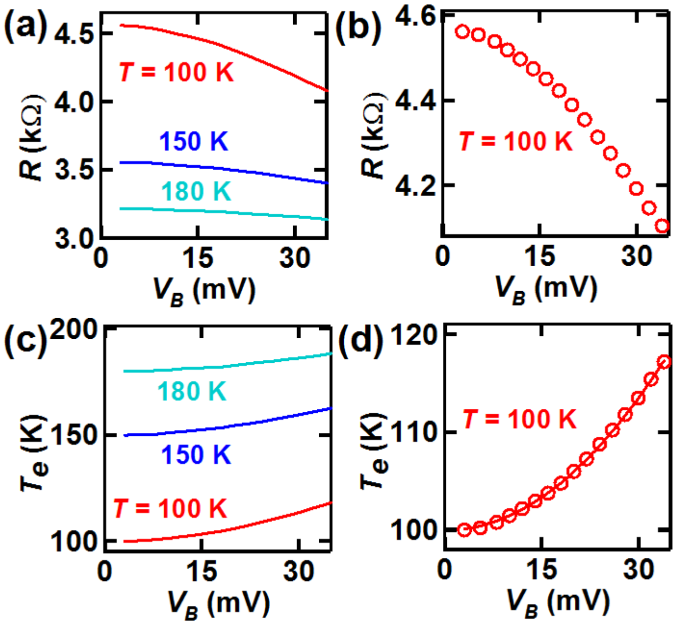


Figure S4: Electron heating for Sample C. (a) $R$ vs $V_B$ at $T$ = 100, 150, 180 K for Device C at $V_G$ = 0.0 V ≈ $V_D$. (b) Zoom-in on the 100 K data. Joule heating due to $V_B$ raises the flake's average $T_e$ above $T$. $T_e$ is extracted using Fig. 2(a). Panels (c) and (d) show $T_e$ vs $V_B$ in Sample B at a few $T$, and at $T$ = 100 K respectively. All of our $K_e$ data is extracted with $V_B \lesssim 30$ mV. The solid line in panel (d) is a power law fit $T_e = 100 + BV_B^x$ , and we find $x$ =2.00 ± 0.02, as expected for Joule heating over a small $T_e$ range.

## 5. Electron-electron scattering length

The electron-electron (inelastic) mean-free path, $l_{ee}$, in graphene was calculated by *Li and Das Sarma* [S3] for various charge densities and temperatures, but for disorder–free samples (ballistic transport). They found that $l_{ee}$ decreases rapidly with $T$. For instance, in their Fig. 3(a) they calculated $l_{ee}$ in suspended graphene at a charge density $n = 10^{10}$ cm$^{-2}$ which is close to the density in our devices (1.7 and 2.1 x $10^{10}$ cm$^{-2}$). They found that $l_{ee} \approx 200$ nm at $T$ = *100 K.* This is shorter than our devices, but only by a factor of 2 or 3. However, the $l_{ee}$ in our devices should be much shorter due to disorder (measured from the width of the $R$-$V_G$ peak). Quoting *Li and Das Sarma* (conclusion): "It is well known that disorder has qualitative and quantitative effects on the inelastic mean free path and the phase breaking length, in general, suppressing the mean free path substantially from its ballistic limit."

Another piece of evidence supporting that $l_{ee}$ in our devices is much shorter than their total length is shown in Fig. S5 where we observe a small, but clearly visible, mesoscopic oscillation in the $G$-$V_G$ characteristic of Sample B at $T$ = 17 K. This oscillation disappears as $T$ is raised above $T$ = 30 K. Mesoscopic oscillations (quantum interferences) are expected when $l_{ee}$ is much longer than $l_{e\text{-}imp}$, and should disappear when $l_{ee} \lesssim l_{e\text{-}imp}$. Thus, Fig. S5 suggests that $l_{ee} \lesssim l_{e\text{-}imp}$ at $T \gtrsim 30$ *K*. Since $l_{e\text{-}imp}$ is significantly shorter than the size of the sample (see main text, and SM section 2), we

expect the same to hold for $l_{ee}$. We do not observe mesoscopic fluctuations in our 3 devices over the $T$ range where we report $K_e$. We also note that *Du et al.* [S4] studied samples which are very similar to ours (length of 0.5 micron, suspended, current annealed, and showing similar mobility and elastic mean-free path), and also observed that mesoscopic fluctuations disappeared above $T \approx 20 - 40$ K (see their Fig. 3(c)). Finally, the agreement between our experimentally extracted and theoretically calculated $K_e$, over the entire $T$ range studied, strongly supports a well defined $T_e(x)$.

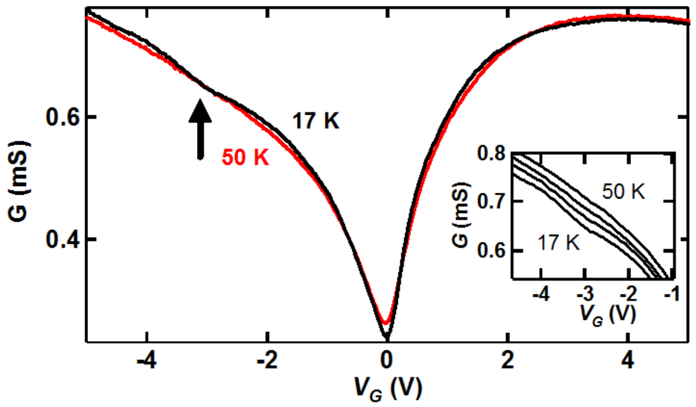


Figure S5: Mesoscopic conductance oscillation in Sample B. $G$ vs $V_G$ at $T$ = 17 and 50 K for Device B. The black arrow indicates a conductance oscillation which disappears at $T$ > 30 K, suggesting that the inelastic mean-free path (due to *e-e* collisions) is comparable to the elastic mfp (e-impurity collisions) in this sample around 30 K. The inset shows $G$ vs $V_G$ at several $T$ between 17 K and 50 K, the curves are offset for clarity.

We also note that since the graphene which is buried under the gold contacts was not current annealed, it is much more disordered that the suspended portion of the device. This large increase in disorder should lead to a reduced $l_{ee}$ under the gold, implying that $l_{ee\text{-}under} < l_{ee\text{-}exposed}$.

## 6. Error analysis

To calculate the uncertainties on the values extracted for $K_e$, using Eq. S3 below, we account for four sources of uncertainty: error on the sample's length, $\Delta L$, width $\Delta W$, resistance $\Delta R$ due to the contact resistance $R_C$, and extracted electronic temperature $\Delta T_e$. We estimate $\Delta L \approx 40$ nm, $\Delta W \approx 50$ nm, $\Delta R = R_C = R_0$ (which is an upper limit since $R_0 = R_C$ + resistance from neutral scatterers), and $\Delta T_e$ = the standard deviation of $T_e$ from the fit of $T_e$ vs $V_B$ as shown in Figs. 3(d), S2(d) and S3(d). We note that the uncertainty $\Delta T_e$ is inversely proportional to the slope of the calibration curve, Fig. 2(a), at $T_e$.

$$K_e = \frac{RI^2L}{12Wh\Delta T} \qquad \text{(S3)}$$

The error on the measured current $I$ is negligible compared to the other sources of error, and the thickness $h = 0.335$ nm is a standard value used by all experiments and theory.

Note that $\Delta T = T_e - T$ where $T$ is the cryostat temperature. The error on $T$ is about 0.1 K and comes from the accuracy of our temperature controller, thus the error on $\Delta T$ is roughly $\Delta T_e$ + 0.1K. We calculate $\Delta K_e$ using Eq. S4,

$$\frac{\Delta K_e}{K_e} = \sqrt{\left(\frac{\Delta L}{L}\right)^2 + \left(\frac{\Delta W}{W}\right)^2 + \left(\frac{\Delta R}{R}\right)^2 + \left(\frac{\Delta(\Delta T)}{\Delta T}\right)^2} \quad \text{(S4)}$$

The calculated errors are shown in Fig. 4. For example, the error bars $\Delta K_e/K_e$ at $T$ = 100 K are 18.3 %, 24.1% and 25.8% from Samples A, B, and C.

## 7. Specific heat calculation

We calculate the charge carrier specific heat, $C_e = \frac{dU_e}{dT}$, where the total energy of the charged quasiparticles, $U_e$, is calculated from the density of states and Dirac statistic for quasiparticles in graphene as,

$$U_e = \int_0^\infty \frac{2\epsilon^2}{\pi(\hbar v_F)^2} \frac{1}{e^{(\epsilon-\mu)/kT}+1}\, d\epsilon - \int_{-\infty}^0 \frac{2\epsilon^2}{\pi(\hbar v_F)^2}\left(\frac{1}{e^{(\epsilon-\mu)/kT}+1} - 1\right) d\epsilon \quad \text{(S5)}$$

where $\mu = \mu_{eff}(T=0) = \hbar v_F \sqrt{\pi n_{tot}(T=0)}$ = 14.8, 15.4 and 17.1 meV are the effective chemical potential for Samples A, B and C respectively. $n_{tot}$ is defined above in Eq. S1 and includes both the gate induced charge density and the impurity induced density.

## 8. Electron cooling length estimate

*Bistritzer and MacDonald* [S5] calculated the electron-acoustic phonon scattering rate for graphene in the intrinsic regime. They found,

$$\gamma_{e-ac} = 1.18 \times 10^3\, D^2\ (\text{meV}^2.\text{s})^{-1} * (k_B T_e)^2 \quad \text{(S6)}$$

where $D$ is the deformation potential measured in eV. The value of $D$ is not well known and has been reported in the range of 10 – 50 eV. We set $D$ = 20 eV, as in Ref. S5 and most other theoretical work. We find $\gamma_{e-ac}$ = 1.7 x $10^6$ – 1.2 x $10^8$ $s^{-1}$ for Sample A over the studied $T_e$ range, 3.2 x $10^6$ – 3.3 x $10^8$ $s^{-1}$ for Sample B, and 2.4 x $10^7$ – 1.6 x $10^8$ $s^{-1}$ for Sample C. Based on these scattering rates, we can estimate the electron cooling length as

$$\xi = \sqrt{\frac{K_e}{\gamma_{e-ac} C_e}} \quad \text{(S7)}$$

Where $K_e$ is the measured heat conductivity in Fig. 4, and $C_e$ the calculated specific heat from section 7 (above). We find $\xi$ = 150 to 14 μm for Sample A, $\xi$ = 74 to 8.5 μm

for Sample B, and $\xi = 27$ to 11 μm for sample C over the $T_e$ range in Fig. 4. These values are always much larger than the length of the devices, 650 nm for A and 400 nm for B and C, which ensures that most of the Joule heating stays in the charge carriers until they reach the gold contacts.

## REFERENCES


[S1] E. V. Castro, *et al.*, *Phys. Rev. Lett.* **105**, 266601 (2010).

[S2] V. E. Dorgan, M. H. Bae, and E. Pop, *Appl. Phys. Lett.* **97**, 082112 (2010).

[S3] Q. Li, and S. Das Sarma, *Phys. Rev. B* **87**, 085406 (2013).

[S4] X. Du, I. Skachko, A. Barker, E. Y. Andrei, *Nature Nanotech*., **3**, 491 (2008).

[S5] R. Bistritzer and A. H. MacDonald, *Phys. Rev. Lett.* **102**, 203410 (2009).
